# Supplementary material for: Search for Neutrino-Induced Neutral Current $\Delta$ Radiative Decay in MicroBooNE and a First Test of the MiniBooNE Low Energy Excess Under a Single-Photon Hypothesis
Source: arXiv:2110.00409 ancillary file (2022-06-20)
Supplement: Supplementary file 1 [file Supplementary_Materials__for_microboone_NCDelta_PRL.pdf]

# Supplemental Materials: Search for Neutrino-Induced Neutral Current $\Delta$ Radiative Decay in MicroBooNE and a First Test of the MiniBooNE Low Energy Excess Under a Single-Photon Hypothesis

## I. NEUTRAL CURRENT $\pi^0$ SELECTION

The NC $\pi^0$ selection targets two event samples: $2\gamma 1p$ and $2\gamma 0p$. The two photons correspond to those expected from $\pi^0$ decay, while the proton (or lack thereof) corresponds to a proton (or neutron) exiting the nucleus. After topological selection requiring exactly one or zero Pandora-reconstructed track(s) and exactly two reconstructed showers, a series of "pre-selection" cuts are applied to remove obvious backgrounds or misreconstructed events from each sample. Those include minimum shower energy requirements of 30 MeV for the leading shower and 20 MeV for the subleading shower in both selections, and a fiducialization cut requiring the reconstructed neutrino vertex and shower start points to be at least 5 cm away from the active TPC volume boundary. For the $2\gamma 1p$ pre-selection, we additionally require that each shower have a conversion distance of at least 1 cm relative to the vertex, and that the track starting point be within 10 cm of the neutrino vertex position. The latter rejects poorly reconstructed events, e.g. due to unresponsive wire regions.

After pre-selection, remaining backgrounds are rejected following the same approach as for the $1\gamma$ final selections. For each selection, a tailored BDT trained on simulated BNB neutrino interactions is used to differentiate NC $\pi^0$ signal (defined as a NC interaction with one $\pi^0$ in the final state) from background interactions based on reconstructed kinematic, geometric, and calorimetric variables. The BDT score cut is optimized for each event sample independently to maximize the product of signal efficiency and signal purity in the final selection.

The resulting reconstructed $\pi^0$ invariant mass distributions are shown in Fig. 1. For the $2\gamma 1p$ final selected event sample, the BDT score cut signal efficiency is 69.9%, with a signal purity of 63.5%, while for the $2\gamma 0p$ event sample, the efficiency and purity are 54.8% and 59.6%, respectively. The efficiencies at all stages can be found in Table I. A Gaussian-plus-linear fit is performed to each distribution to extract the reconstructed $\pi^0$ invariant mass. For the $2\gamma 1p$ event sample, this fit gives a mean value of 138.9±2.1 MeV/$c^2$ with a width of 31.7±2.4 MeV$c^2$. For $2\gamma 0p$, the extracted mean is 143.3±3.2 MeV$c^2$ with a width of 47.9±4.9 MeV$c^2$.

An overall data deficit relative to the MC nominal prediction suggests an overestimate of the NC $\pi^0$ rate normalizations in GENIE. Nevertheless, the observed difference is within the assigned flux uncertainties and cross-section uncertainties within GENIE, and is assumed to be well-characterized by those uncertainties and correlations across all samples used in the analysis: $1\gamma 1p$, $1\gamma 0p$, $2\gamma 1p$ and $2\gamma 0p$.

| Selection Stage | $2\gamma 1p$ eff. | $2\gamma 0p$ eff. |
|---|---|---|
| Topological | 10.5% | 6.60% |
| Pre-selection | 59.4% | 77.3% |
| BDT Selection | 69.9% | 54.8% |
| Combined | 4.36% | 2.81% |

TABLE I. NC $\pi^0$ efficiencies for the $2\gamma 1p$ and $2\gamma 0p$ selections. The topological and combined efficiencies are evaluated relative to all true NC $1\pi^0$ events inside the active TPC. The pre-selection and BDT selection efficiencies are evaluated relative to their respective preceding selection stage.

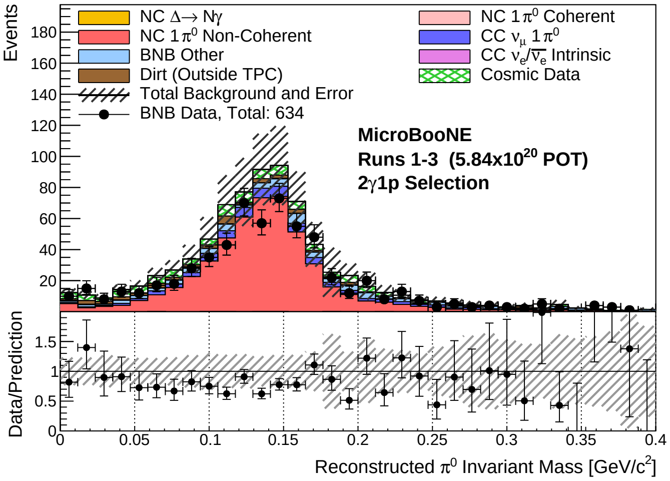


(a) $2\gamma 1p$

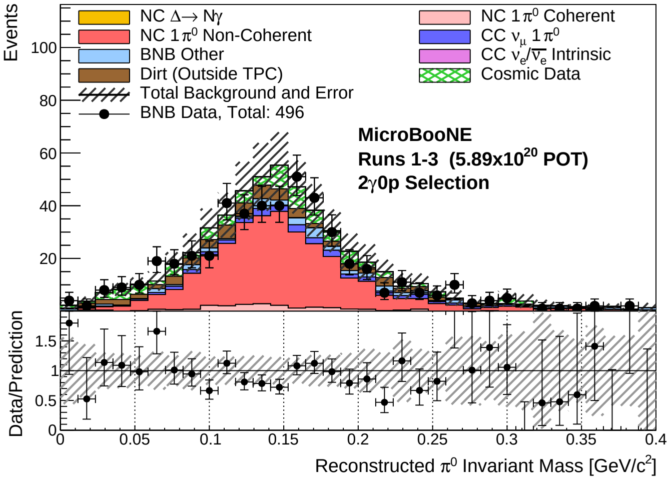


(b) $2\gamma 0p$

FIG. 1. The reconstructed $\pi^0$ invariant mass distributions for the final selected $2\gamma 1p$ and $2\gamma 0p$ event samples.

| Selection | Bin Number | $E_\gamma^{reco}$ Range [GeV] | $p_{\pi^0}^{reco}$ Range [GeV/$c$] | Background CV | Signal CV | Observed Data |
|---|---|---|---|---|---|---|
| $1\gamma1p$ | 1 | [0,0.6) | - | 26.98 | 4.88 | 16 |
| $1\gamma0p$ | 2 | [0.1,0.7) | - | 165.35 | 6.55 | 153 |
| $2\gamma1p$ | 3 | - | [0, 0.15) | 185.69 | 0.14 | 154 |
| | 4 | - | [0.15, 0.225) | 179.49 | 0.21 | 155 |
| | 5 | - | [0.225, 0.3) | 137.88 | 0.19 | 105 |
| | 6 | - | [0.3, 0.375) | 100.51 | 0.13 | 83 |
| | 7 | - | [0.375, 0.45) | 72.68 | 0.07 | 53 |
| | 8 | - | [0.45, 0.6) | 81.36 | 0.08 | 55 |
| | 9 | - | [0.6, 0.9) | 34.03 | 0.04 | 23 |
| $2\gamma0p$ | 10 | - | [0, 0.15) | 98.17 | 0.11 | 92 |
| | 11 | - | [0.15, 0.225) | 105.05 | 0.09 | 114 |
| | 12 | - | [0.225, 0.3) | 100.10 | 0.07 | 101 |
| | 13 | - | [0.3, 0.375) | 87.23 | 0.07 | 72 |
| | 14 | - | [0.375, 0.45) | 60.87 | 0.05 | 50 |
| | 15 | - | [0.45, 0.6) | 63.38 | 0.05 | 48 |
| | 16 | - | [0.6, 0.9) | 27.92 | 0.02 | 18 |

TABLE II. Data and predicted number of events per bin for the final selected $1\gamma1p$, $1\gamma0p$, $2\gamma1p$ and $2\gamma0p$ distributions used in the $x_\Delta$ fit. Events in the $1\gamma$ selections are binned in terms of reconstructed photon shower energy, while events in the $2\gamma$ selections are binned in terms of reconstructed $\pi^0$ momentum. Signal NC $\Delta \to N\gamma$ events contribute negligibly in the $2\gamma$ final selected event samples.

## II. FINAL SELECTED PREDICTIONS AND OBSERVED DATA

The predicted number of events per bin for the final selected $1\gamma1p$, $1\gamma0p$, $2\gamma1p$ and $2\gamma0p$ distributions used in the $x_\Delta$ fit are summarized in Table II, broken down in terms of signal (corresponding to the nominal, GENIE-predicted NC $\Delta \to N\gamma$) and background, along with corresponding bin boundaries. The fit is performed over one (1) bin of reconstructed shower energy, $E_\gamma^{reco}$, for each of the $1\gamma$ selections, and seven (7) bins of reconstructed $\pi^0$ momentum, $p_{\pi^0}^{reco}$, for each of the $2\gamma$ selections. The observed data per bin after final selection are also provided, for the same binning.

## III. SYSTEMATIC COVARIANCE MATRIX

The fractional systematic covariance matrix, including bin-by-bin systematic uncertainties and systematic correlations for the final $1\gamma1p$, $1\gamma0p$, $2\gamma1p$, and $2\gamma0p$ selections, is shown in Fig. 2. The covariance matrix is provided in terms of $16 \times 16$ bins, corresponding to one (1) bin of reconstructed shower energy for each of the $1\gamma$ distributions, and seven (7) bins of reconstructed $\pi^0$ momentum for each of the $2\gamma$ distributions. The systematic covariance matrix includes flux, cross-section, Geant4, detector, and nominal MC simulation intrinsic statistical uncertainty, due to the finite MC statistics. GENIE uncertainty on $\mathcal{B}_{\text{eff}}(\Delta \to N\gamma)$ is not included in the analysis. The fractional systematic covariance matrix is also provided in Table III. Please note that the fractional covariance matrix is inclusive of signal uncertainties and correlations corresponding to the nominal GENIE-predicted NC $\Delta \to N\gamma$ event rate in Table II.

The covariance matrix provided in Table III can be used to calculate the $\chi^2$ between the observed data and the nominal MC prediction. For readers interested in reproducing the fit result shown in this article, by performing a fit to the normalization ($x_\Delta$) of the nominal rate of NC $\Delta \to N\gamma$, a $18 \times 18$-bin fractional systematic covariance matrix, including the same systematic uncertainties, is provided in Table IV, with 18 bins corresponding to one (1) bin of reconstructed shower energy for signal and one (1) bin of reconstructed shower energy for background, for each of the $1\gamma$ distributions, and seven (7) bins of reconstructed $\pi^0$ momentum for each of the $2\gamma$ distributions. Signal (NC $\Delta \to N\gamma$) is not separated out from background for the $2\gamma$ distributions in this covariance matrix, for simplicity, as those can be approximated as negligible.

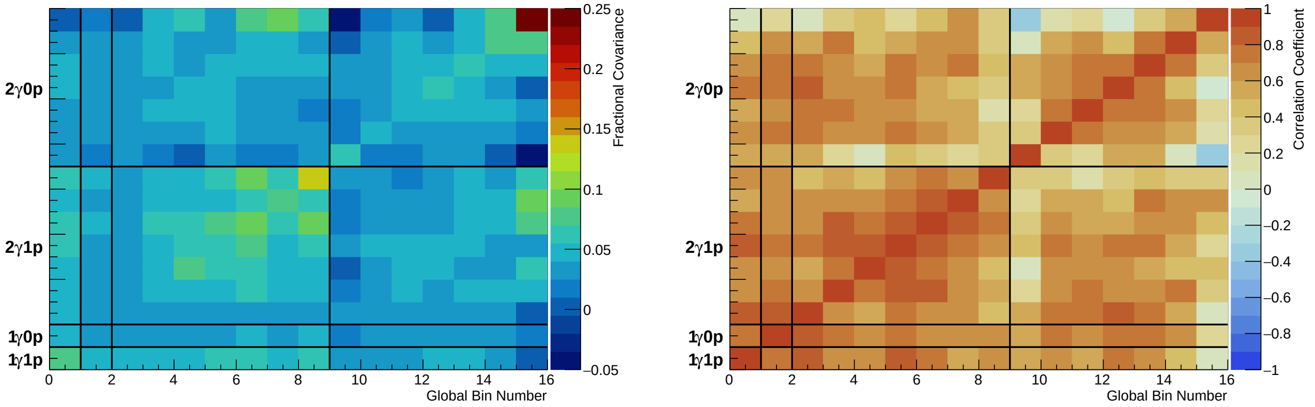


(a) Fractional Systematic Covariance Matrix

(b) Systematic Correlation Matrix

FIG. 2. (a) The total fractional systematic covariance matrix for the final selected $1\gamma 1p$, $1\gamma 0p$, $2\gamma 1p$, and $2\gamma 0p$ event samples, in bins of reconstructed shower energy for the $1\gamma$ distributions, and reconstructed $\pi^0$ momentum for the $2\gamma$ distributions. The bin boundaries are defined in Sec. II. (b) The systematic correlation matrix for the same covariance matrix, highlighting the strong correlations between $1\gamma$ and $2\gamma$ final selected event samples.

| Bin | $1\gamma 1p$ | $1\gamma 0p$ | $2\gamma 1p$ | | | | | | | $2\gamma 0p$ | | | | | | |
|---|---|---|---|---|---|---|---|---|---|---|---|---|---|---|---|---|
| 1 | **0.0817** | 0.0412 | 0.0464 | 0.0432 | 0.0511 | 0.0622 | 0.0628 | 0.0455 | 0.0674 | 0.0358 | 0.0372 | 0.0369 | 0.0536 | 0.0487 | 0.0350 | 0.00610 |
| 2 | 0.0412 | **0.0364** | 0.0298 | 0.0321 | 0.0335 | 0.0375 | 0.0402 | 0.0311 | 0.0442 | 0.0236 | 0.0298 | 0.0297 | 0.0362 | 0.0361 | 0.0360 | 0.0199 |
| 3 | 0.0464 | 0.0298 | **0.0367** | 0.0307 | 0.0316 | 0.0397 | 0.0360 | 0.0308 | 0.0342 | 0.0258 | 0.0295 | 0.0318 | 0.0376 | 0.0355 | 0.0288 | 0.00216 |
| 4 | 0.0432 | 0.0321 | 0.0307 | **0.0544** | 0.0517 | 0.0509 | 0.0596 | 0.0433 | 0.0427 | 0.0141 | 0.0335 | 0.0431 | 0.0340 | 0.0409 | 0.0457 | 0.0413 |
| 5 | 0.0511 | 0.0335 | 0.0316 | 0.0517 | **0.0802** | 0.0603 | 0.0632 | 0.0507 | 0.0499 | 0.00613 | 0.0364 | 0.0450 | 0.0445 | 0.0394 | 0.0353 | 0.0638 |
| 6 | 0.0622 | 0.0375 | 0.0397 | 0.0509 | 0.0603 | **0.0691** | 0.0715 | 0.0531 | 0.0593 | 0.0269 | 0.0417 | 0.0418 | 0.0463 | 0.0491 | 0.0386 | 0.0389 |
| 7 | 0.0628 | 0.0402 | 0.0360 | 0.0596 | 0.0632 | 0.0715 | **0.0943** | 0.0672 | 0.0857 | 0.0240 | 0.0389 | 0.0381 | 0.0384 | 0.0538 | 0.0502 | 0.0729 |
| 8 | 0.0455 | 0.0311 | 0.0308 | 0.0433 | 0.0507 | 0.0531 | 0.0672 | **0.0710** | 0.0645 | 0.0166 | 0.0331 | 0.0332 | 0.0298 | 0.0504 | 0.0447 | 0.0903 |
| 9 | 0.0674 | 0.0442 | 0.0342 | 0.0427 | 0.0499 | 0.0593 | 0.0857 | 0.0645 | **0.133** | 0.0322 | 0.0290 | 0.0119 | 0.0318 | 0.0405 | 0.0355 | 0.0620 |
| 10 | 0.0358 | 0.0236 | 0.0258 | 0.0141 | 0.00613 | 0.0269 | 0.0240 | 0.0166 | 0.0322 | **0.0606** | 0.0191 | 0.0153 | 0.0334 | 0.0318 | 0.00636 | -0.0397 |
| 11 | 0.0372 | 0.0298 | 0.0295 | 0.0335 | 0.0364 | 0.0417 | 0.0389 | 0.0331 | 0.0290 | 0.0191 | **0.0435** | 0.0343 | 0.0332 | 0.0345 | 0.0318 | 0.0191 |
| 12 | 0.0369 | 0.0297 | 0.0318 | 0.0431 | 0.0450 | 0.0418 | 0.0381 | 0.0332 | 0.0119 | 0.0153 | 0.0343 | **0.0541** | 0.0414 | 0.0445 | 0.0440 | 0.0264 |
| 13 | 0.0536 | 0.0362 | 0.0376 | 0.0340 | 0.0445 | 0.0463 | 0.0384 | 0.0298 | 0.0318 | 0.0334 | 0.0332 | 0.0414 | **0.0577** | 0.0454 | 0.0320 | -0.000191 |
| 14 | 0.0487 | 0.0361 | 0.0355 | 0.0409 | 0.0394 | 0.0491 | 0.0538 | 0.0504 | 0.0405 | 0.0318 | 0.0345 | 0.0445 | 0.0454 | **0.0640** | 0.0514 | 0.0483 |
| 15 | 0.0350 | 0.0360 | 0.0288 | 0.0457 | 0.0353 | 0.0386 | 0.0502 | 0.0447 | 0.0355 | 0.00636 | 0.0318 | 0.0440 | 0.0320 | 0.0514 | **0.0738** | 0.0718 |
| 16 | 0.00610 | 0.0199 | 0.00216 | 0.0413 | 0.0638 | 0.0389 | 0.0729 | 0.0903 | 0.0620 | -0.0397 | 0.0191 | 0.0264 | -0.000191 | 0.0483 | 0.0718 | **0.250** |

TABLE III. The fractional systematic covariance matrix for the final selected $1\gamma 1p$, $1\gamma 0p$, $2\gamma 1p$, and $2\gamma 0p$ event samples, in bins of reconstructed shower energy for the $1\gamma$ distributions, and reconstructed $\pi^0$ momentum for the $2\gamma$ distributions. The bin boundaries are defined in Sec. II. All variances have been rounded to three significant digits. Bin-diagonal variances are highlighted in bold.

| Bin | $1\gamma 1p$ | | $1\gamma 0p$ | | $2\gamma 1p$ | | | | | | | $2\gamma 0p$ | | | | | | |
|---|---|---|---|---|---|---|---|---|---|---|---|---|---|---|---|---|---|---|
| | Sig | Bkg | Sig | Bkg | | | | | | | | | | | | | | |
| 1 | **0.0738** | 0.0623 | 0.0567 | 0.0359 | 0.0412 | 0.0374 | 0.0368 | 0.0471 | 0.0496 | 0.0422 | 0.0526 | 0.0286 | 0.0296 | 0.0349 | 0.0476 | 0.0473 | 0.0413 | 0.0118 |
| 2 | 0.0623 | **0.0891** | 0.0483 | 0.0417 | 0.0473 | 0.0442 | 0.0537 | 0.0650 | 0.0651 | 0.0461 | 0.0701 | 0.0371 | 0.0386 | 0.0372 | 0.0547 | 0.0490 | 0.0338 | 0.00507 |
| 3 | 0.0567 | 0.0483 | **0.0630** | 0.0326 | 0.0309 | 0.0405 | 0.0461 | 0.0463 | 0.0564 | 0.0484 | 0.0538 | 0.0160 | 0.0272 | 0.0359 | 0.0415 | 0.0483 | 0.0461 | 0.0552 |
| 4 | 0.0359 | 0.0417 | 0.0326 | **0.0367** | 0.0297 | 0.0318 | 0.0330 | 0.0372 | 0.0396 | 0.0305 | 0.0438 | 0.0239 | 0.0299 | 0.0294 | 0.0360 | 0.0356 | 0.0356 | 0.0185 |
| 5 | 0.0412 | 0.0473 | 0.0309 | 0.0297 | **0.0367** | 0.0307 | 0.0316 | 0.0397 | 0.0360 | 0.0308 | 0.0342 | 0.0258 | 0.0295 | 0.0318 | 0.0376 | 0.0355 | 0.0288 | 0.00216 |
| 6 | 0.0374 | 0.0442 | 0.0405 | 0.0318 | 0.0307 | **0.0544** | 0.0517 | 0.0509 | 0.0596 | 0.0433 | 0.0427 | 0.0141 | 0.0335 | 0.0431 | 0.0340 | 0.0409 | 0.0457 | 0.0413 |
| 7 | 0.0368 | 0.0537 | 0.0461 | 0.0330 | 0.0316 | 0.0517 | **0.0802** | 0.0603 | 0.0632 | 0.0507 | 0.0499 | 0.00613 | 0.0364 | 0.0450 | 0.0445 | 0.0394 | 0.0353 | 0.0638 |
| 8 | 0.0471 | 0.0650 | 0.0463 | 0.0372 | 0.0397 | 0.0509 | 0.0603 | **0.0691** | 0.0715 | 0.0531 | 0.0593 | 0.0269 | 0.0417 | 0.0418 | 0.0463 | 0.0491 | 0.0386 | 0.0389 |
| 9 | 0.0496 | 0.0651 | 0.0564 | 0.0396 | 0.0360 | 0.0596 | 0.0632 | 0.0715 | **0.0943** | 0.0672 | 0.0857 | 0.0240 | 0.0389 | 0.0381 | 0.0384 | 0.0538 | 0.0502 | 0.0729 |
| 10 | 0.0422 | 0.0461 | 0.0484 | 0.0305 | 0.0308 | 0.0433 | 0.0507 | 0.0531 | 0.0672 | **0.0710** | 0.0645 | 0.0166 | 0.0331 | 0.0332 | 0.0298 | 0.0504 | 0.0447 | 0.0903 |
| 11 | 0.0526 | 0.0701 | 0.0538 | 0.0438 | 0.0342 | 0.0427 | 0.0499 | 0.0593 | 0.0857 | 0.0645 | **0.133** | 0.0322 | 0.0290 | 0.0119 | 0.0318 | 0.0405 | 0.0355 | 0.0620 |
| 12 | 0.0286 | 0.0371 | 0.0160 | 0.0239 | 0.0258 | 0.0141 | 0.00613 | 0.0269 | 0.0240 | 0.0166 | 0.0322 | **0.0606** | 0.0191 | 0.0153 | 0.0334 | 0.0318 | 0.00636 | -0.0397 |
| 13 | 0.0296 | 0.0386 | 0.0272 | 0.0299 | 0.0295 | 0.0335 | 0.0364 | 0.0417 | 0.0389 | 0.0331 | 0.0290 | 0.0191 | **0.0435** | 0.0343 | 0.0332 | 0.0345 | 0.0318 | 0.0191 |
| 14 | 0.0349 | 0.0372 | 0.0359 | 0.0294 | 0.0318 | 0.0431 | 0.0450 | 0.0418 | 0.0381 | 0.0332 | 0.0119 | 0.0153 | 0.0343 | **0.0541** | 0.0414 | 0.0445 | 0.0440 | 0.0264 |
| 15 | 0.0476 | 0.0547 | 0.0415 | 0.0360 | 0.0376 | 0.0340 | 0.0445 | 0.0463 | 0.0384 | 0.0298 | 0.0318 | 0.0334 | 0.0332 | 0.0414 | **0.0577** | 0.0454 | 0.0320 | -0.000191 |
| 16 | 0.0473 | 0.0490 | 0.0483 | 0.0356 | 0.0355 | 0.0409 | 0.0394 | 0.0491 | 0.0538 | 0.0504 | 0.0405 | 0.0318 | 0.0345 | 0.0445 | 0.0454 | **0.0640** | 0.0514 | 0.0483 |
| 17 | 0.0413 | 0.0338 | 0.0461 | 0.0356 | 0.0288 | 0.0457 | 0.0353 | 0.0386 | 0.0502 | 0.0447 | 0.0355 | 0.00636 | 0.0318 | 0.0440 | 0.0320 | 0.0514 | **0.0738** | 0.0718 |
| 18 | 0.0118 | 0.00507 | 0.0552 | 0.0185 | 0.00216 | 0.0413 | 0.0638 | 0.0389 | 0.0729 | 0.0903 | 0.0620 | -0.0397 | 0.0191 | 0.0264 | -0.000191 | 0.0483 | 0.0718 | **0.250** |

TABLE IV. The fractional systematic covariance matrix for the final selected $1\gamma 1p$, $1\gamma 0p$, $2\gamma 1p$, and $2\gamma 0p$ event samples, in bins of reconstructed shower energy for the $1\gamma 1p$ signal, $1\gamma 1p$ background, $1\gamma 0p$ signal and $1\gamma 0p$ background distributions, and reconstructed $\pi^0$ momentum for the $2\gamma$ distributions. The bin boundaries are defined in Sec. II. All variances have been rounded to three significant digits. Bin-diagonal variances are highlighted in bold.

## IV. EFFECTIVE BRANCHING FRACTION

The reinterpretation of the normalization $x_\Delta$ as a scaling of the effective branching fraction $\mathcal{B}_{\rm eff}(\Delta \to N\gamma)$ is further illustrated in Fig. 3. Here, the nominal prediction ($x_\Delta = 1$) corresponds to an effective branching fraction of 0.6%, where the NC $\Delta \to N\gamma$ rate in GENIE is parametrized as a function of the off-shell $\Delta$ invariant mass, $W$. This effective branching fraction can be thought of as a metric to account for any unknown nuclear or BSM effects that might modify the $\Delta$ behavior inside the nuclear medium.

## V. EFFICIENCIES

The signal efficiencies for the $1\gamma$ selections are provided in Fig. 4a, defined as the ratio of all selected signal events relative to all true NC $\Delta \to N\gamma$ events whose true interaction vertex is inside the active TPC. The latter corresponds to 124.1 expected events for $6.80 \times 10^{20}$ POT. The figures highlight that the existence of a track (proton candidate) allows for higher efficiency for photons of lower (true) energy. Shown in Fig. 4b is the same information for the NC $\pi^0$-rich $2\gamma$ selections, as a function of true $\pi^0$ momentum, showing the same qualitative trends.

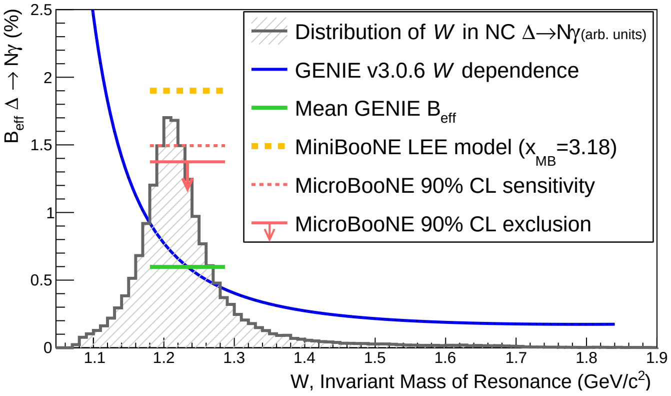


FIG. 3. The extracted 90% CL on the effective branching fraction of neutrino-induced NC $\Delta \to N\gamma$. The gray shaded histogram shows the distribution of $W$, the resonance invariant mass, for all simulated NC $\Delta \to N\gamma$. At low $W$, when the $\Delta$ is further off-shell, the dominant decay $\Delta \to N\pi^0$ becomes suppressed due to phase space effects around the $N\pi^0$ threshold, leading to an increased effective branching fraction to $N\gamma$. This is modeled in GENIE via the $W$-dependence as shown by the blue curve.

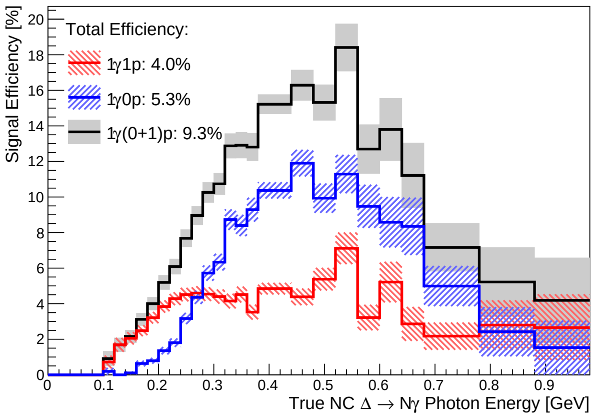


(a)

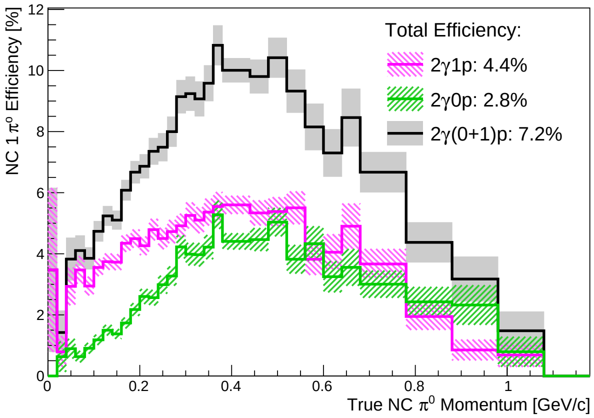


(b)

FIG. 4. (a) The signal NC $\Delta \to N\gamma$ efficiency as a function of true photon energy, for $1\gamma 1p$, $1\gamma 0p$ and the joint $1\gamma(0+1)p$ selections. (b) NC $1\pi^0$ efficiency as a function of true $\pi^0$ momentum, for the high-statistics $2\gamma 1p$, $2\gamma 0p$ and the joint $2\gamma(0+1)p$ selections.
